# Supplementary material for: Second order perturbation theory to determine the magnetic state of finite size aromatic hydrocarbons molecules
Source: arXiv:1705.08474 source file (2017-06-29)
Supplement: Supplementary file 1 [file Supplementary_material1.pdf]

# SUPPLEMENTARY MATERIAL (1) FOR "SECOND ORDER PERTURBATION THEORY TO DETERMINE THE MAGNETIC STATE OF FINITE SIZE AROMATIC HYDROCARBONS MOLECULES"

Usually first- and second-order Rayleigh-Schrödinger perturbation theory is used in condensed matter starting from the large interaction limit where the kinetic energy is used as a perturbation[1]. In this appendix we show how to treat the electronic repulsion as a weak perturbation (the general formalism is exposed in refs. 2 and 3).

On the main text we use the Hubbard model[4] to describe the electronic interactions in conjugated systems. The model Hamiltonian contains a non-interacting part $\hat{H}_0$ and a term that incorporates the on-site electron-electron interaction $\hat{H}_1$:

$$\hat{H} = \hat{H}_0 + \hat{H}_1. \tag{1}$$

The non-interacting part is a tight-binding Hamiltonian,

$$\hat{H}_0 = -t \sum_{i,j;\sigma} \left( \hat{c}^\dagger_{i\sigma} \hat{c}_{j\sigma} + \hat{c}^\dagger_{j\sigma} \hat{c}_{i\sigma} \right), \tag{2}$$

that describe the kinetic energy with a constant hopping $t$ between sites $i$ and $j$. The interacting part of $\hat{H}$ is

$$\hat{H}_1 = U \sum_{i=1}^{N} (\hat{n}_{i\uparrow} - 1/2)(\hat{n}_{i\downarrow} - 1/2), \tag{3}$$

where $U$ is the on-site Coulomb interaction and $N$ denote the number of sites. $N_{e,\sigma}$ is the number of electrons with spin $\sigma$ in the system.

Let us call $\hat{c}_{p\sigma}$ the operators that diagonalize $\hat{H}_0$. The original annihilation site operators are written as a linear combination of these operators as

$$\hat{c}_{i\sigma} = \sum_{p'} \beta_{p'\sigma,i} \hat{c}_{p'\sigma}. \tag{4}$$

In the limit of weakly correlated electrons we treat the interaction as a small perturbation in the total energy. The energy of a state can be written as $E = E^{(0)} + \lambda\alpha + \lambda^2\beta + O(\lambda^3)$ where $\lambda = U/t$. The energy for the unperturbed system is simply the energy of a tight-binding model

$$E^{(0)} = \langle n^{(0)} | \hat{H}_0 | n^{(0)} \rangle, \tag{5}$$

where

$$|n^{(0)}\rangle = \prod_{p_\uparrow \in S_{n,\uparrow}, p_\downarrow \in S_{n,\downarrow}} \hat{c}^\dagger_{p_\downarrow} \hat{c}^\dagger_{p_\uparrow} |0\rangle \tag{6}$$

is a state of the unperturbed system, which can easily be obtained once $\hat{H}_0$ is exactly diagonalizable. $S_{n,\sigma}$ is a set of eigenstates of $\hat{H}_0$ labelled by $p\sigma$ ($\sigma = \uparrow, \downarrow$) with energy $\varepsilon_{p_\sigma}$.

The first-order Rayleigh-Schrödinger perturbation teory correction for the energy is

$$\lambda\alpha = \langle n^{(0)}|\hat{H}_1|n^{(0)}\rangle. \tag{7}$$

The Rayleigh-Schrödinger second-order perturbation term at non-degenerate state $|n^{(0)}\rangle$ is

$$\lambda^2\beta = \sum_{k \neq n} \frac{|\langle n^{(0)}|\hat{H}_1|k^{(0)}\rangle|^2}{E_n^{(0)} - E_k^{(0)}}, \tag{8}$$

where $|k^{(0)}\rangle \neq |n^{(0)}\rangle$ is a state of the unperturbed system. The diagonal part of $\hat{H}_1$, proportional to the constant term $-U/2N$, does not introduce any contribution to the second-order correction for the energy. In this expression only the correlation term $U\hat{n}_{i\uparrow}\hat{n}_{i\downarrow}$, not diagonal in the $k$ basis, contributes to the energy correction at second-order.

We write the non-interacting state $|n^{(0)}\rangle$ or $|k^{(0)}\rangle$ as the direct product of up and down states

$$|n^{(0)}\rangle = |n_\uparrow^{(0)}\rangle|n_\downarrow^{(0)}\rangle, \tag{9}$$

$$|k^{(0)}\rangle = |k_\uparrow^{(0)}\rangle|k_\downarrow^{(0)}\rangle. \tag{10}$$

For the second-order correction Eq. (8) we need to compute

$$\begin{aligned}\langle k^{(0)}|\hat{H}_1|n^{(0)}\rangle &= \langle k^{(0)}|U\sum_{i=1}^{N}\hat{n}_{i\uparrow}\hat{n}_{i\downarrow}|n^{(0)}\rangle \\ &= U\sum_{i=1}^{N}\langle k^{(0)}|\hat{n}_{i\uparrow}\hat{n}_{i\downarrow}|n^{(0)}\rangle\end{aligned} \tag{11}$$

Using Eqs. (9) and (10)

$$\begin{aligned}\langle k^{(0)}|\hat{H}_1|n^{(0)}\rangle &= U\sum_{i=1}^{N}\langle k_\downarrow^{(0)}|\langle k_\uparrow^{(0)}|\hat{n}_{i\uparrow}\hat{n}_{i\downarrow}|n_\uparrow^{(0)}\rangle|n_\downarrow^{(0)}\rangle \\ &= U\sum_{i=1}^{N}\langle k_\uparrow^{(0)}|\hat{n}_{i\uparrow}|n_\uparrow^{(0)}\rangle\langle k_\downarrow^{(0)}|\hat{n}_{i\downarrow}|n_\downarrow^{(0)}\rangle\end{aligned} \tag{12}$$

Evaluating one of these mean values for the generic spin variable $\sigma$ we have

$$\langle k_\sigma^{(0)}|\hat{n}_\sigma|n_\sigma^{(0)}\rangle = (\langle 0| \prod_{q\in S_{k,\sigma}} \hat{c}_{q\sigma})\hat{c}_{i\sigma}^\dagger \hat{c}_{i\sigma}( \prod_{q'\in S_{n,\sigma}} \hat{c}_{q'\sigma}^\dagger|0\rangle).$$

Using Eq. (4) we write this expression as

$$\begin{aligned}\langle k_\sigma^{(0)}|\hat{n}|n_\sigma^{(0)}\rangle &= \langle 0| \prod_{q\in S_{k,\sigma}} \hat{c}_{q\sigma} \sum_{pp'} \beta_{p'\sigma i}\beta_{p\sigma i}^* \hat{c}_{p\sigma}^\dagger \hat{c}_{p'\sigma} \prod_{q'\in S_{n,\sigma}} \hat{c}_{q'\sigma}^\dagger|0\rangle \\ &= \sum_{pp'} \beta_{p'\sigma i}\beta_{p\sigma i}^* \langle 0| \prod_{q\in S_{k,\sigma}} \hat{c}_{q\sigma}\hat{c}_{p\sigma}^\dagger \hat{c}_{p'\sigma} \prod_{q'\in S_{n,\sigma}} \hat{c}_{q'\sigma}^\dagger|0\rangle.\end{aligned} \tag{13}$$

For this mean value to be different from zero in any case $p'$ must belong to $S_n$ and there are two possibilities for $p$:

- $p = p'$ implying that $S_{k,\sigma} = S_{n,\sigma}$ so $\langle k_\sigma^{(0)}| = \langle n_\sigma^{(0)}|$. The Eq. (14) then resumes to

$$\sum_{p=p'\in S_{n,\sigma}} |\beta_{p_\sigma i}|^2 = \langle n_\sigma^{(0)}|\hat{n}_{i\sigma}|n_\sigma^{(0)}\rangle = \langle \hat{n}_{i\sigma}\rangle \tag{14}$$

  and the energy of the state $|k_\sigma^{(0)}\rangle$ is $E_{k\sigma}^{(0)} = E_{n\sigma}^{(0)} = \langle n_\sigma^{(0)}|\hat{H}_0|n_\sigma^{(0)}\rangle$.

- If $p \neq p'$, then $p$ must not belong to $S_{n\sigma}$. Then Eq. (14) becomes

$$\langle k_\sigma^{(0)}|\hat{n}_\sigma|n_\sigma^{(0)}\rangle = \beta_{p'_\sigma i}\beta_{p_\sigma i}^* \tag{15}$$

  and $S_{k,\sigma}$ must contains all the elements of $S_{n,\sigma}$ that include $p$ and exclude $p'$. The energy of the state $|k_\sigma^{(0)}\rangle$ is $E_{k\sigma}^{(0)} = E_{n\sigma}^{(0)} + \varepsilon_{p\sigma} - \varepsilon_{p'\sigma}$.

The condition $|k^{(0)}\rangle \neq |n^{(0)}\rangle$ can be written as $|k_\uparrow^{(0)}\rangle|k_\downarrow^{(0)}\rangle \neq |n_\uparrow^{(0)}\rangle|n_\downarrow^{(0)}\rangle$. This last condition can be satisfied in three cases

I . $|k_\uparrow^{(0)}\rangle \neq |n_\uparrow^{(0)}\rangle \wedge |k_\downarrow^{(0)}\rangle \neq |n_\downarrow^{(0)}\rangle$

II . $|k_\uparrow^{(0)}\rangle \neq |n_\uparrow^{(0)}\rangle \wedge |k_\downarrow^{(0)}\rangle = |n_\downarrow^{(0)}\rangle$

III . $|k_\uparrow^{(0)}\rangle = |n_\uparrow^{(0)}\rangle \wedge |k_\downarrow^{(0)}\rangle \neq |n_\downarrow^{(0)}\rangle$

Taking into considerations these possibilities Eq. (8) becomes

$$\lambda^2\beta = U^2(\beta_0 + \beta_\uparrow + \beta_\downarrow) \tag{16}$$

where $\beta_0$ is the term obtained when $|k_\uparrow^{(0)}\rangle \neq |n_\uparrow^{(0)}\rangle$ and $|k_\downarrow^{(0)}\rangle \neq |n_\downarrow^{(0)}\rangle$

$$\beta_0 = \sum_{i,j} \sum_{\substack{p'_\uparrow \in S_{n\uparrow}, p'_\downarrow \in S_{n\downarrow} \\ p_\uparrow \notin S_{n\uparrow}, p_\downarrow \notin S_{n\downarrow}}} \frac{\beta^*_{p'\uparrow,j}\beta_{p\uparrow,j}\beta^*_{p'\downarrow,j}\beta_{p\downarrow,j}\beta^*_{p'\uparrow,i}\beta_{p\uparrow,i}\beta^*_{p'\downarrow,i}\beta_{p\downarrow,i}}{\varepsilon_{p\uparrow} + \varepsilon_{p\downarrow} - \varepsilon_{p'\uparrow} - \varepsilon_{p'\downarrow}} \tag{17}$$

$$= \sum_{\substack{p'_\uparrow \in S_{n\uparrow}, p'_\downarrow \in S_{n\downarrow} \\ p_\uparrow \notin S_{n\uparrow}, p_\downarrow \notin S_{n\downarrow}}} \frac{\left[\sum_j \beta^*_{p'j\uparrow}\beta_{pj\uparrow}\beta^*_{p'j\downarrow}\beta_{pj\downarrow}\right]^2}{\varepsilon_{p\uparrow} + \varepsilon_{p\downarrow} - \varepsilon_{p'\uparrow} - \varepsilon_{p'\downarrow}}.$$

$\beta_\uparrow$ is the term obtained when $|k_\uparrow^{(0)}\rangle \neq |n_\uparrow^{(0)}\rangle$ and $|k_\downarrow^{(0)}\rangle = |n_\downarrow^{(0)}\rangle$

$$\beta_\uparrow = \sum_{i,j} \sum_{\substack{p'_\uparrow \in S_{n\uparrow} \\ p_\uparrow \notin S_{n\uparrow}}} \frac{\beta^*_{p'\uparrow,j}\beta_{p\uparrow,j}\beta^*_{p'\uparrow,i}\beta_{p\uparrow,i}\langle \hat{n}_{j\downarrow}\rangle\langle \hat{n}_{i\downarrow}\rangle}{\varepsilon_{p\uparrow} - \varepsilon_{p'\uparrow}} \tag{18}$$

$$= \sum_{\substack{p'_\uparrow \in S_{n\uparrow} \\ p_\uparrow \notin S_{n\uparrow}}} \frac{[\sum_j \beta^*_{p'\uparrow,j}\beta_{p\uparrow,j}\langle \hat{n}_{j\downarrow}\rangle]^2}{\varepsilon_{p\uparrow} - \varepsilon_{p'\uparrow}}$$

$\beta_\downarrow$ is completely analogous to $\beta_\uparrow$.

$$\beta_\downarrow = \sum_{\substack{p'_\downarrow \in S_{n\downarrow} \\ p_\downarrow \notin S_{n\downarrow}}} \frac{[\sum_j \beta^*_{p'\downarrow,j}\beta_{p\downarrow,j}\langle \hat{n}_{j\downarrow}\rangle]^2}{\varepsilon_{p\downarrow} - \varepsilon_{p'\downarrow}} \tag{19}$$

The last fourth equations give the second-order perturbation correction to the energy of the state $|n^{(0)}\rangle$ due to $\hat{H}_1$.

A Maxima [5] script to perform these calculations is found in supplementary material (2), the executable script is made available on requesting to the authors.

---


[1] D. Khomskii, *Basic Aspects of the Quantum Theory of Solids: Order and Elementary Excitations* (Cambridge University Press, 2010).

[2] J. Sakurai and J. Napolitano, *Modern Quantum Mechanics*, 2nd ed. (Addison-Wesley, 2011).

[3] tagkey1981169, in *Second Quantization-Based Methods in Quantum Chemistry*, edited by P. Jørgensen and J. Simons (Academic Press, 1981) pp. 169 – 172.

[4] J. Hubbard, in *Proceedings of the Royal Society of London A: Mathematical, Physical and Engineering Sciences*, Vol. 276 (The Royal Society, 1963) pp. 238–257.

[5] Maxima Open-source Computer Algebra Systems Maxima; software available at http://maxima.sourceforge.net.
