# Supplementary material for: Second order perturbation theory to determine the magnetic state of finite size aromatic hydrocarbons molecules
Source: arXiv:1705.08474 source file (2017-06-29)

# SUPPLEMENTARY MATERIAL (2) FOR ”SECOND ORDER PERTURBATION THEORY TO DETERMINE THE MAGNETIC STATE OF FINITE SIZE AROMATIC HYDROCARBONS MOLECULES”

## 1 to set the number of azulene oligomers at the system

Nsit defines the number of atoms at the system

```
-> NumberOfOligomers: 2 $ Nsit : 10 + ( NumberOfOligomers - 1)*8; t: 1.$
```

18

## 2 to create a matrix, OliMatrix, for the non interacting Hamiltonian

```
-> modulo( a, b ) :=a - b*floor( a/b )$
-> OliMatrix:zeromatrix(Nsit, Nsit) $
-> for i: 1 thru Nsit do for j: 1 thru Nsit do if i-j = 1 and modulo(i,8)=7 then
   OliMatrix[i,j]:-t else if i-j = -1 and modulo(i,8) = 1 then OliMatrix[i,j]:-t else if
   i-j = 2 then OliMatrix[i,j]:-t;
-> auxMat:OliMatrix + transpose(OliMatrix)$ OliMatrix:auxMat$
```

## 3 compute the eiguenvalues and eigenvectors of the unperturbed system

```
-> load (lapack)$
-> eigenSys: dgeev ( OliMatrix ,True)$
-> eigenvalues: eigenSys[1]$
-> eigenvectors: transpose ( eigenSys[2] ) $
```

# 4 Tight-binding calculation for the electronic density of the non-perturbated system

–> orderedeigenvalues : sort (eigenvalues) $

FermiGround defines the Fermi level, FermiP1 and FeermiM1 set the eletronic filling for first excited state

–> FermiGround : orderedeigenvalues[Nsit/2]; FermiP1 : orderedeigenvalues[Nsit/2 + 1]$ FermiM1 : orderedeigenvalues[Nsit/2 - 1]$

–> sitedensity (i, FermiLevel) := sum ( if eigenvalues[j] <= FermiLevel then eigenvectors[j][i]ˆ2 else 0, j, 1, Nsit)$

–> density : makelist ( [ i , 2. * sitedensity(i,FermiGround)] , i, Nsit)$

densDn and densUp compute respectively the density of electrons with spin up and down

–> densDn : makelist ([ i , sitedensity(i,FermiM1)], i, Nsit)$ densUp : makelist ([ i , sitedensity(i,FermiP1)], i, Nsit)$

densUpDnMs0 is density of electrons with spin up and down compputed on Ms = 0 spin projections sub - spaces

–> densUpDnMs0 : makelist ( sitedensity(i,FermiGround)*sitedensity(i,FermiGround), i, Nsit)$

densUpDnMs1 is density of electrons with spin up and down compputed on Ms = 1 spin projections sub - spaces

–> densUpDnMs1 : makelist ( sitedensity(i,FermiP1)*sitedensity(i,FermiM1), i, Nsit)$

# 5 energies of the unperturbated system on Ms = 0 and Ms=1 spin projections sub - spaces

–> energyMs0 : 2. * sum ( if eigenvalues[j] <= FermiGround then eigenvalues[j] else 0, j, 1, Nsit);

$$-24.52188174203637$$

–> energyMs1 : energyMs0 + FermiP1 -FermiGround;

$$-24.01615315026958$$

## 6 First-Order Perturbation Theory for the Hubbard model on Ms=0 and Ms=1 spin projections sub-spaces

Eq.(7) at SUPPLEMENTARY MATERIAL (1) compputed on Ms=0 spin projections sub-spaces

```
--> alfaMs0 : sum ( densUpDnMs0[i], i, 1, Nsit) - Nsit/2.;
```

$$-4.449986242244303$$

Eq.(7) at SUPPLEMENTARY MATERIAL (1) compputed on Ms=1 spin projections sub-spaces

```
--> alfaMs1 : sum ( densUpDnMs1[i], i, 1, Nsit) - Nsit/2.;
```

$$-4.557368647201192$$

Uc is the critical value of the electronic correlation for First-Order Perturbation Theory

```
--> float ( solve ( [ Uc * ( alfaMs1 - alfaMs0 ) - ( energyMs1 - energyMs0)], [Uc]) ) ;
```

$$[Uc = -4.709603886873415]$$

## 7 Second-Order Perturbation Theory for the Hubbard model on Ms=0 spin projections sub-space

SumBB is the numerator in Eq.(17) at supplementary material (1)

```
--> SumBB (ppu,pu,ppd,pd) := if eigenvalues[ppu] <= FermiGround and eigenvalues[pu] > FermiGround and eigenvalues[ppd] <= FermiGround and eigenvalues[pd] > FermiGround then sum ( eigenvectors[ppu][j]*eigenvectors[pu][j]*eigenvectors[ppd][j]*eigenvectors[pd][j] , j, 1, Nsit) else 0$
```

SumBB is the denominator in Eq.(17) at supplementary material (1)

```
–> DeltaE (ppu, pu, ppd, pd) := if eigenvalues[ppu] <= FermiGround and eigenvalues[pu] > FermiGround and eigenvalues[ppd] <= FermiGround and eigenvalues[pd] > FermiGround then eigenvalues[pu] + eigenvalues[pd] - eigenvalues[ppu] - eigenvalues[ppd] else 10000$
```

To build a table, TableBBEner, for the fraction at Eq.(17 )

```
–> array (TableBBEner, flonum, Nsit, Nsit, Nsit, Nsit,2);
–> for ppu: 1 thru Nsit do for pu: 1 thru Nsit do for ppd: 1 thru Nsit do for pd: 1 thru Nsit do TableBBEner[ppu,pu,ppd,pd,1]:SumBB(ppu, pu, ppd, pd)^2$
–> for ppu: 1 thru Nsit do for pu: 1 thru Nsit do for ppd: 1 thru Nsit do for pd: 1 thru Nsit do TableBBEner[ppu,pu,ppd,pd,2]:DeltaE(ppu, pu, ppd, pd)$
```

Eq.(17) at supplementary material (1)

```
–> beta0 : sum ( sum ( sum ( sum ( TableBBEner[ppu,pu,ppd,pd,1]/ TableBBEner[ppu,pu,ppd,pd,2], pd,1,Nsit) , ppd,1,Nsit), pu,1,Nsit) , ppu,1,Nsit)$
```

DeltaEUp is the denominator in Eq.(18) at supplementary material (1)

```
–> DeltaEUp (ppu, pu) := if eigenvalues[ppu] <= FermiGround and eigenvalues[pu] > FermiGround then eigenvalues[pu] - eigenvalues[ppu] else 10000$
```

SumBBNd is the numerator in Eq.(18) at supplementary material (1)

```
–> SumBBNd (ppu,pu) := if eigenvalues[ppu] <= FermiGround and eigenvalues[pu] > FermiGround then sum ( eigenvectors[ppu][j]*eigenvectors[pu][j]* 1./2. * density[j][2] , j, 1, Nsit) else 0$
```

To build a table, TableBUNdEner, for the fraction at Eq.(18)

```
–> array (TableBUNdEner, flonum, Nsit, Nsit,2)$
–> for ppu: 1 thru Nsit do for pu: 1 thru Nsit do TableBUNdEner[ppu,pu,1]:SumBBNd(ppu,pu)^2;
–> for ppu: 1 thru Nsit do for pu: 1 thru Nsit do TableBUNdEner[ppu,pu,2]:DeltaEUp(ppu, pu);
```

Eq.(18) at supplementary material (1)

```
–> betaUp : sum ( sum ( TableBUNdEner[ppu,pu,1]/ TableBUNdEner[ppu,pu,2], pu,1,Nsit) , ppu,1,Nsit)$
```

Eq.(8) at SUPPLEMENTARY MATERIAL (1) comppputed on Ms=0 spin projections sub-spaces

```
-->     betaMs0 : (beta0+2*betaUp);
```

0.28447881854422

EnergyU2Ms0 is the energy of the system computet at Ms = 0 spin projections sub - spaces by using second-order perturbation theory

```
-->     U : 1.0$
-->     energyU2Ms0 : energyMs0+ alfaMs0*U-(betaMs0)*U^2;
```

−29.25634680282489

# 8 Second-Order Perturbation Theory for the Hubbard model on Ms=1 spin projections subspace

SumBB is the numerator in Eq.(17) at supplementary material (1)

```
-->     SumBB (ppu,pu,ppd,pd) := if eigenvalues[ppu] <= FermiP1 and eigenvalues[pu] > FermiP1 and eigenvalues[ppd] < FermiGround and eigenvalues[pd] >= FermiGround then sum ( eigenvectors[ppu][j]*eigenvectors[pu][j]*eigenvectors[ppd][j]*eigenvectors[pd][j] , j, 1, Nsit) else 0$
```

SumBB is the denominator in Eq.(17) at supplementary material (1)

```
-->     DeltaE (ppu, pu, ppd, pd) := if eigenvalues[ppu] <= FermiP1 and eigenvalues[pu] > FermiP1 and eigenvalues[ppd] < FermiGround and eigenvalues[pd] >= FermiGround then eigenvalues[pu] + eigenvalues[pd] - eigenvalues[ppu] - eigenvalues[ppd] else 10000$
```

To build a table, TableBBEner, for the fraction at Eq.(17 )

```
-->     array (TableBBEner, flonum, Nsit, Nsit, Nsit, Nsit,2)$
-->     for ppu: 1 thru Nsit do for pu: 1 thru Nsit do for ppd: 1 thru Nsit do for pd: 1 thru Nsit do TableBBEner[ppu,pu,ppd,pd,1]:SumBB(ppu, pu, ppd, pd)^2;
-->     for ppu: 1 thru Nsit do for pu: 1 thru Nsit do for ppd: 1 thru Nsit do for pd: 1 thru Nsit do TableBBEner[ppu,pu,ppd,pd,2]:DeltaE(ppu, pu, ppd, pd);
```

Eq.(17) at supplementary material (1)

```
–> beta0 : sum ( sum ( sum ( sum ( TableBBEner[ppu,pu,ppd,pd,1]/ TableBBEner[ppu,pu,ppd,pd,2], pd,1,Nsit) , ppd,1,Nsit), pu,1,Nsit) , ppu,1,Nsit);
```

SumBB is the denominator in Eq.(18) at supplementary material (1)

```
–> DeltaEUp (ppu, pu) := if eigenvalues[ppu] <= FermiP1 and eigenvalues[pu] > FermiP1 then eigenvalues[pu] - eigenvalues[ppu] else 10000$
```

SumBB is the numerator in Eq.(18) at supplementary material (1)

```
–> SumBBNd (ppu,pu) := if eigenvalues[ppu] <= FermiP1 and eigenvalues[pu] > FermiP1 then sum ( eigenvectors[ppu][j]*eigenvectors[pu][j]*densDn[j][2] , j, 1, Nsit) else 0$
```

To build a table, TableBUNdEner, for the fraction at Eq.(18 )

```
–> array (TableBUNdEner, flonum, Nsit, Nsit,2);
–> for ppu: 1 thru Nsit do for pu: 1 thru Nsit do TableBUNdEner[ppu,pu,1]:SumBBNd(ppu,pu)^2;
–> for ppu: 1 thru Nsit do for pu: 1 thru Nsit do TableBUNdEner[ppu,pu,2]:DeltaEUp(ppu, pu);
```

Eq.(18) at supplementary material (1)

```
–> betaUp : sum ( sum ( TableBUNdEner[ppu,pu,1]/ TableBUNdEner[ppu,pu,2], pu,1,Nsit) , ppu,1,Nsit);
```

SumBB is the denominator in Eq.(19) at supplementary material (1)

```
–> DeltaEdown (ppd, pd) := if eigenvalues[ppd] < FermiGround and eigenvalues[pd] >= FermiGround then eigenvalues[pd] - eigenvalues[ppd] else 10000$
```

SumBB is the numerator in Eq.(19) at supplementary material (1)

```
–> SumBBNu (ppd,pd) := if eigenvalues[ppd] < FermiGround and eigenvalues[pd] >= FermiGround then sum ( eigenvectors[ppd][j]*eigenvectors[pd][j]*densUp[j][2] , j, 1, Nsit) else 0$
```

To build a table, TableBUNuEner, for the fraction at Eq.(19)

```
–> array (TableBUNuEner, flonum, Nsit, Nsit,2)$
–> for ppd: 1 thru Nsit do for pd: 1 thru Nsit do TableBUNuEner[ppd,pd,1]:SumBBNu(ppd,pd)^2;
–> for ppd: 1 thru Nsit do for pd: 1 thru Nsit do TableBUNuEner[ppd,pd,2]:DeltaEdown(ppd, pd);
```

Eq.(19) at supplementary material (1)

```
-->  betaDn : sum ( sum ( TableBUNuEner[ppd,pd,1]/ TableBUNuEner[ppd,pd,2],
     pd,1,Nsit) , ppd,1,Nsit)$
```

Eq.(8) at SUPPLEMENTARY MATERIAL (1) compputed on Ms=1 spin projections sub-spaces

```
-->  betaMs1 : (beta0+betaUp+betaDn);
```

$$0.27116767746926$$

EnergyU2Ms1 is the energy of the system computet at Ms = 1 spin projections sub - spaces by using second-order perturbation theory

```
-->  U : 1.0$
```

```
-->  energyU2Ms1 : energyMs1+ alfaMs1*U-(betaMs1)*U*U;
```

$$-28.84468947494004$$

# 9 Uc calculations for second-order Perturbation theory

Uc is the ritical value of the electronic correlation U obtained with Second-Order Perturbation Theory

```
-->  float ( solve ( [ -(betaMs1-betaMs0)*Uc2^2+( alfaMs1 - alfaMs0 )*Uc2 + (
     energyMs1 - energyMs0)], [Uc2]) ) ;
```

$$[Uc2 = -5.15148293230098610^{-23}\left(9.04754775038856310^{22}\%i - 7.82988852695616810^{22}\right)$$

$$Uc2 = 5.15148293230098610^{-23}\left(9.04754775038856310^{22}\%i + 7.82988852695616710^{22}\right)]$$

```
-->  wxplot2d([-(betaMs1-betaMs0)*x^2+( alfaMs1 - alfaMs0 )*x + ( energyMs1 -
     energyMs0)], [x,0,5], [y,0,0.5], [box, false], [label, ["x", 5.2, 0.],["Spin Gap", -1.6,
     .3]])$
```

plot2d: some values were clipped.

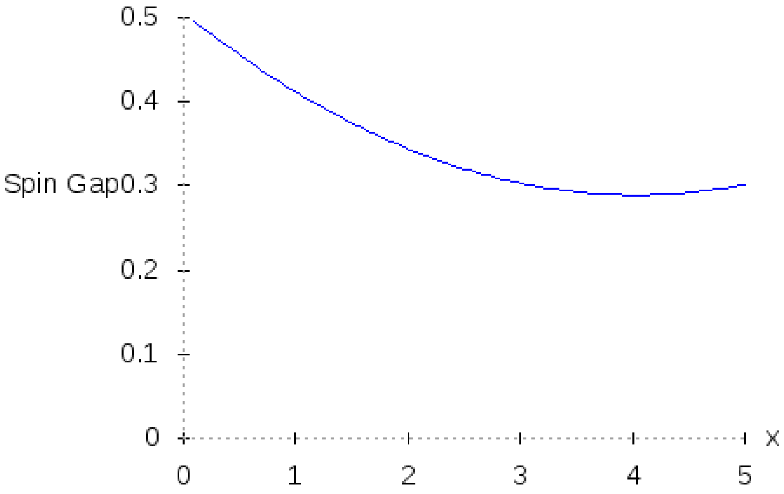

Supplement: Supplementary file 2 [file Supplementary_material2.pdf]
